# Supplementary material for: NamedCurves: Learned Image Enhancement via Color Naming
Source: arXiv:2407.09892 source file (2024-07-13)

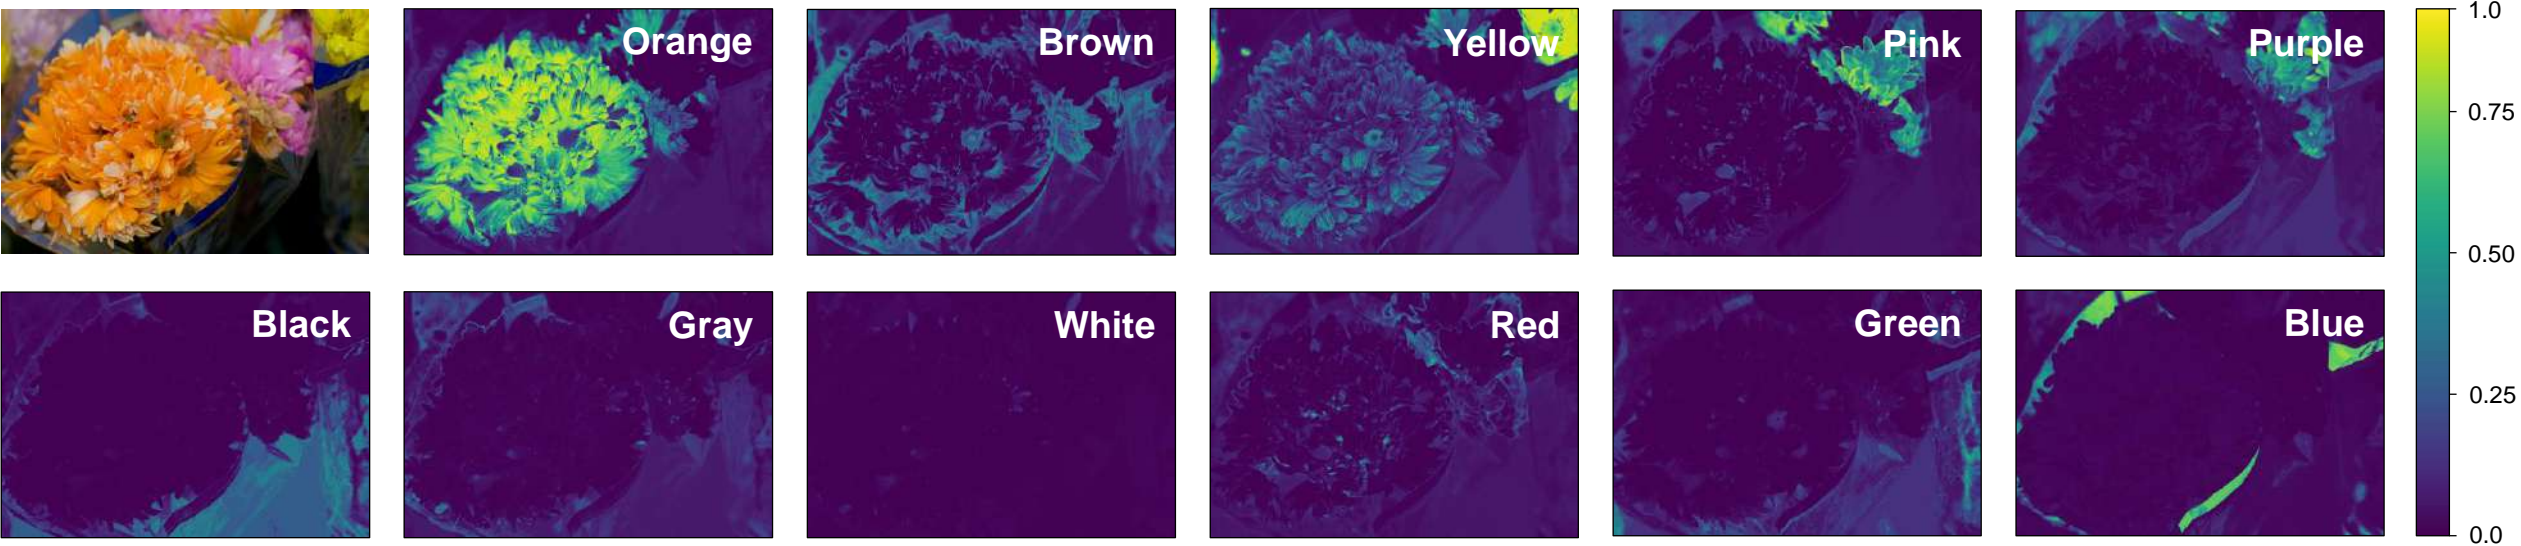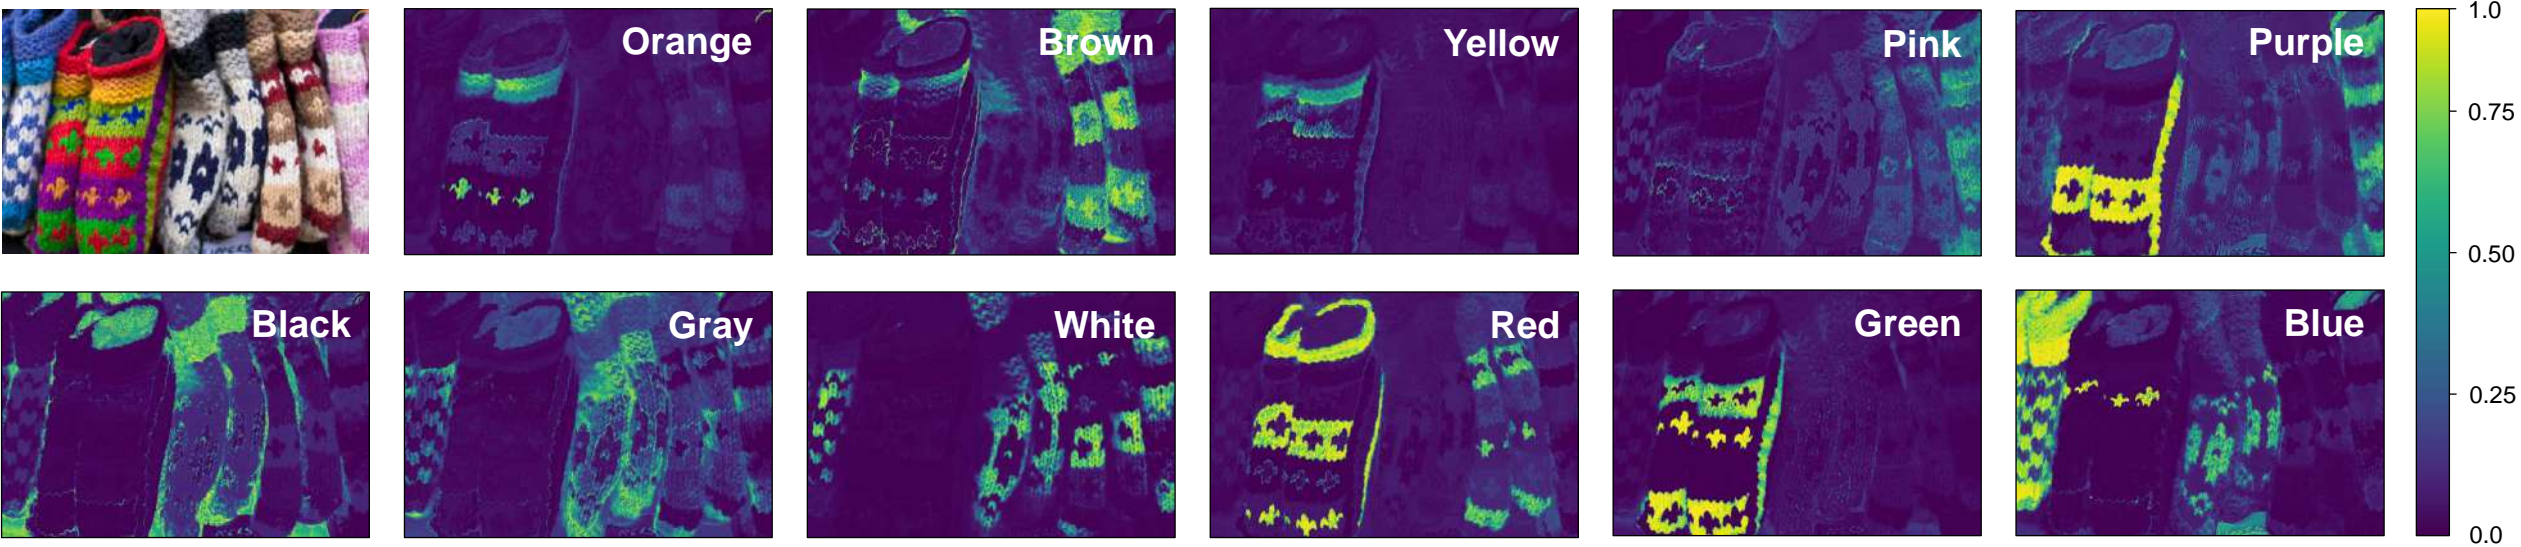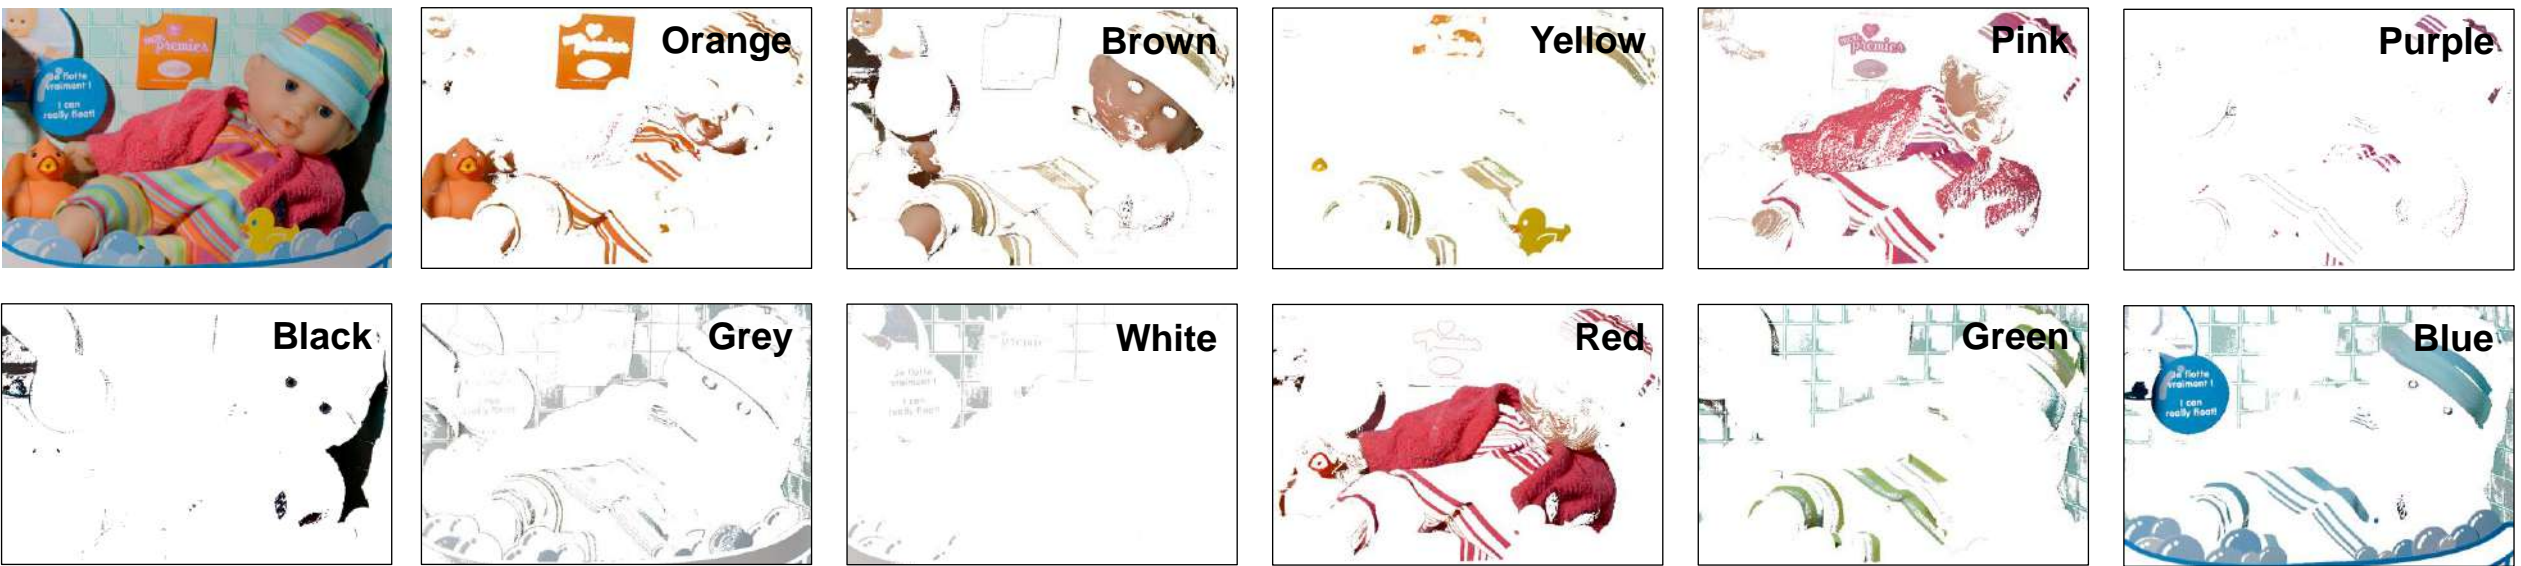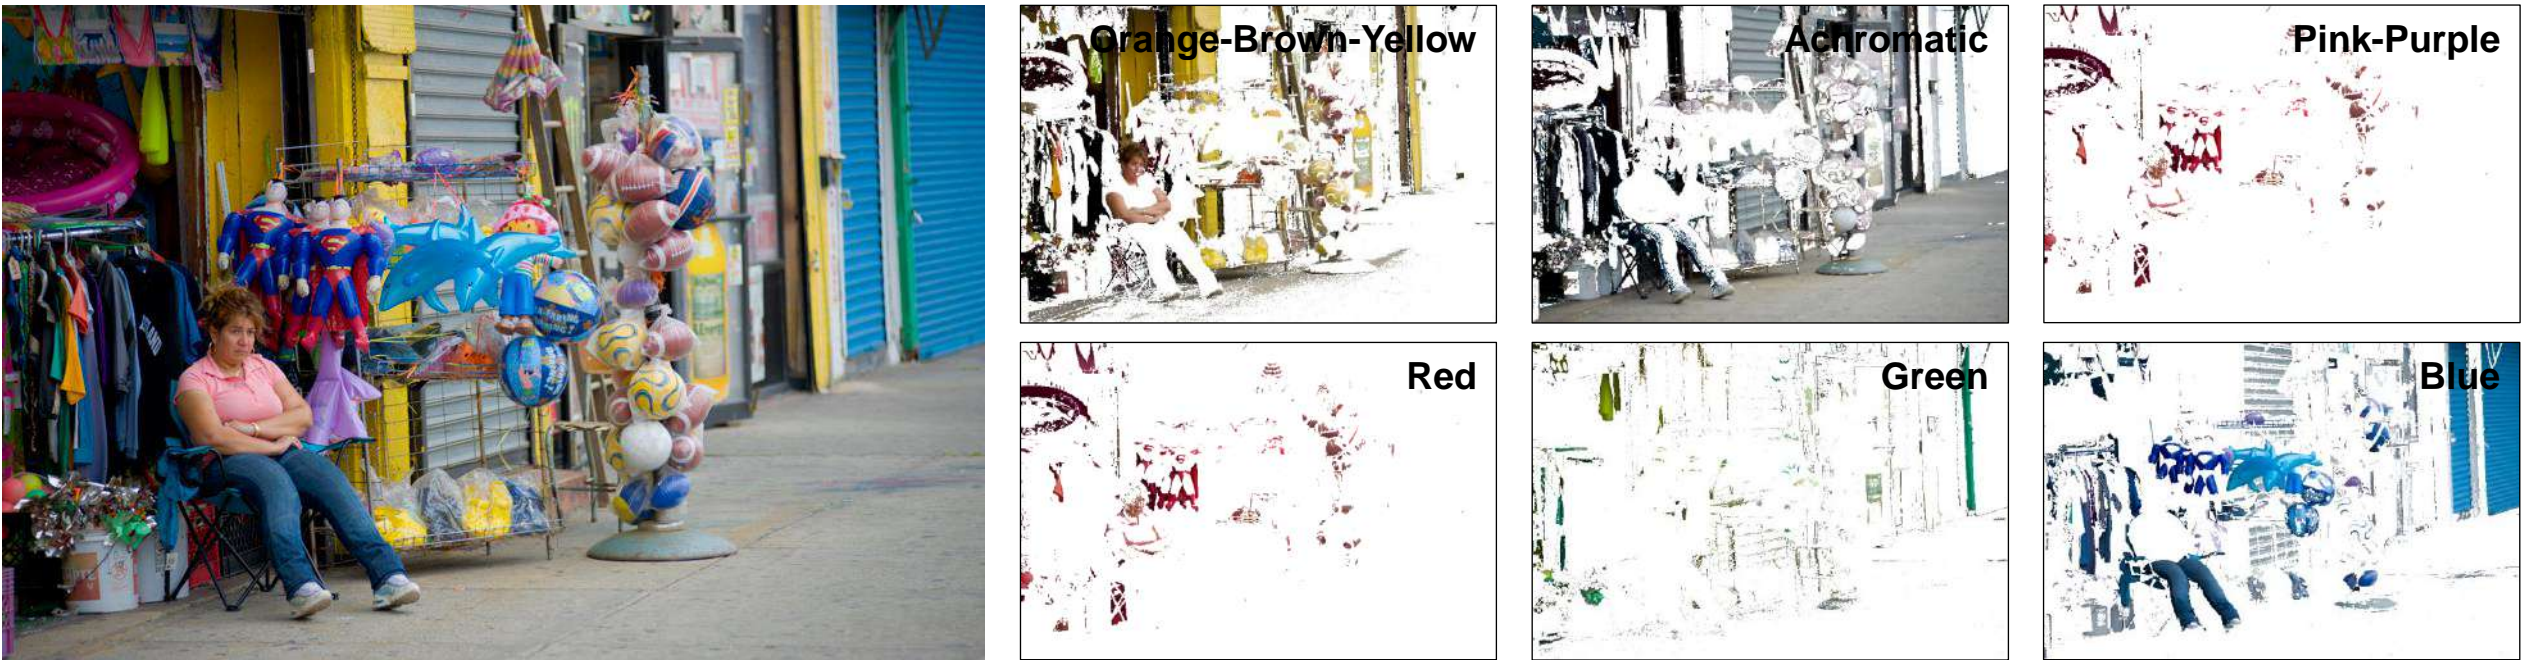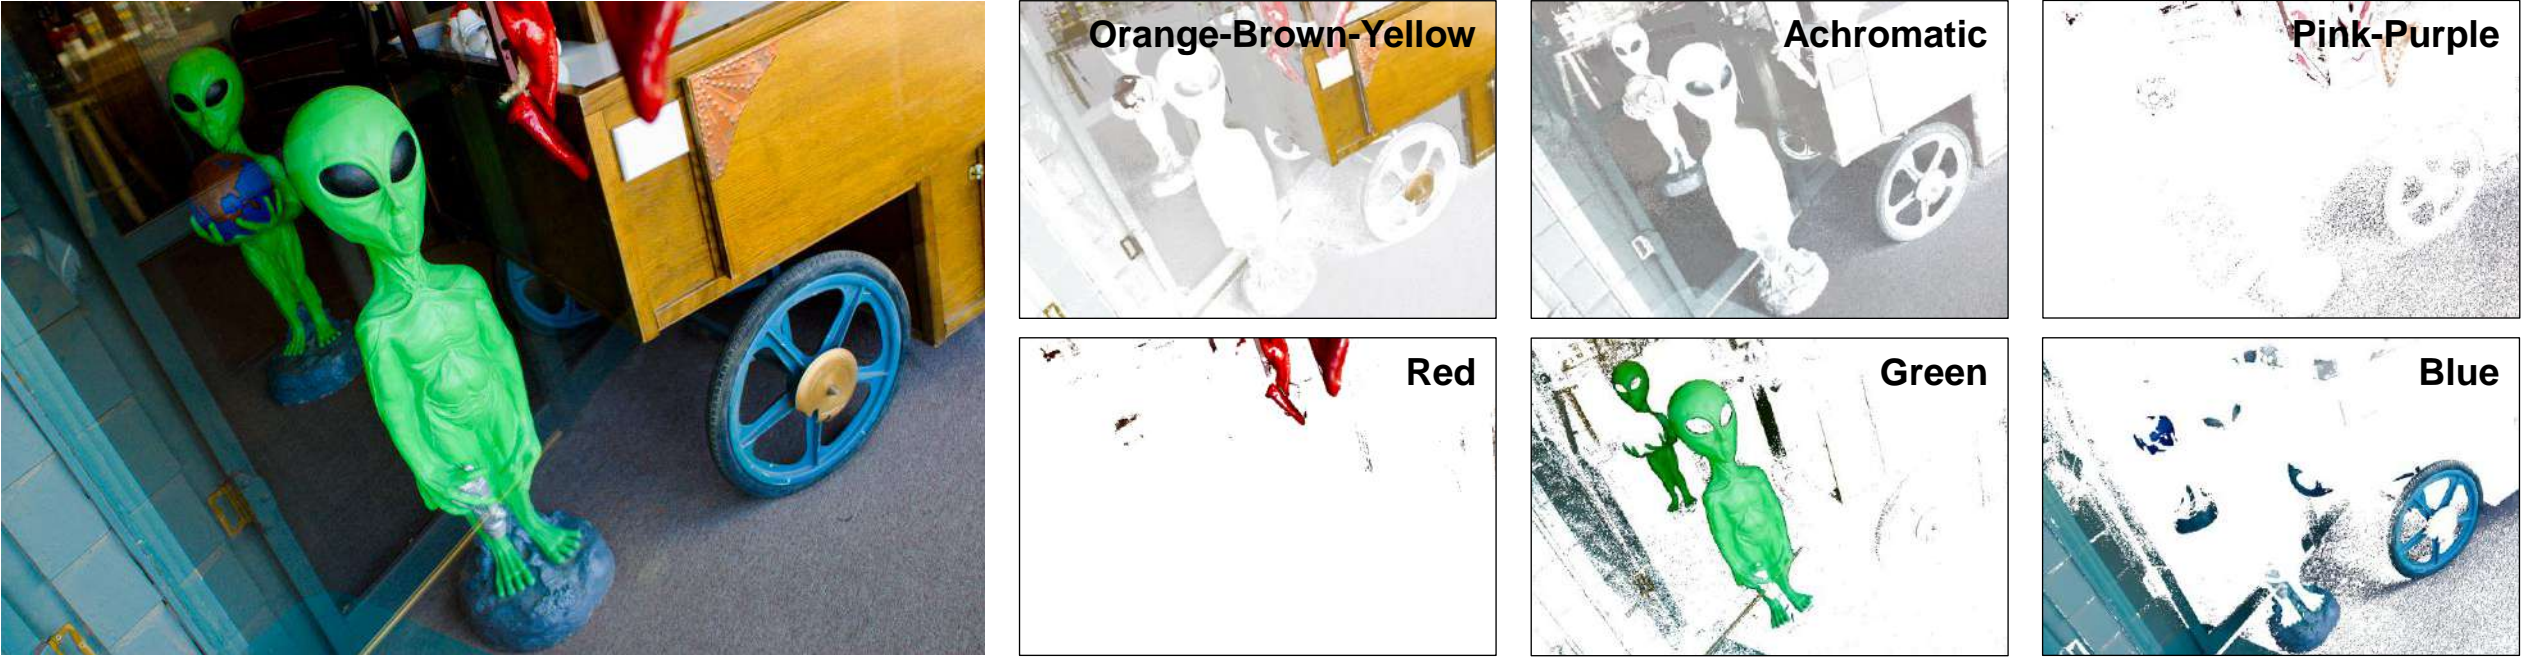



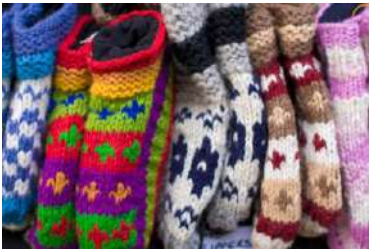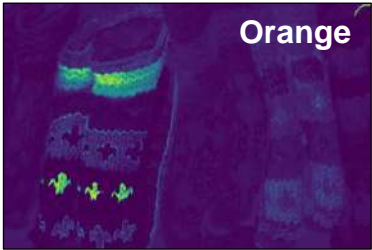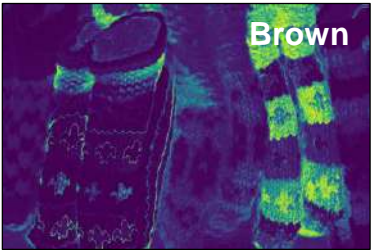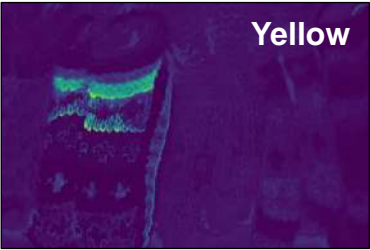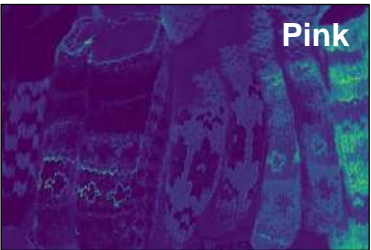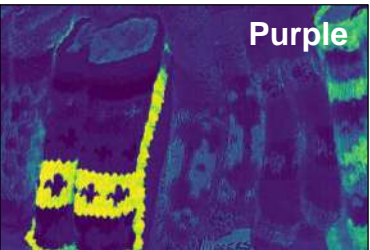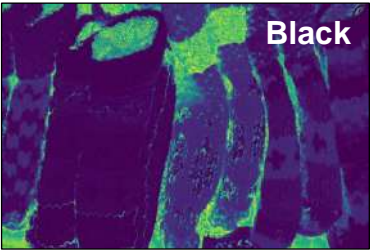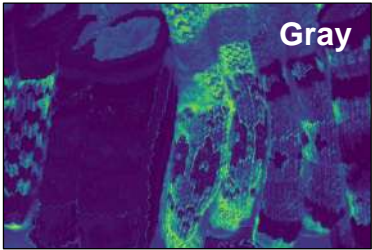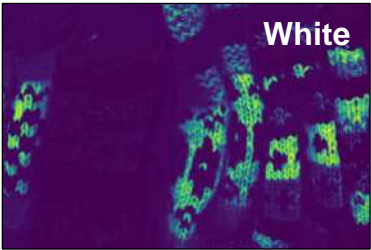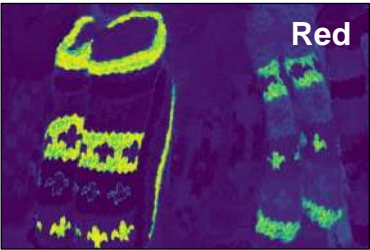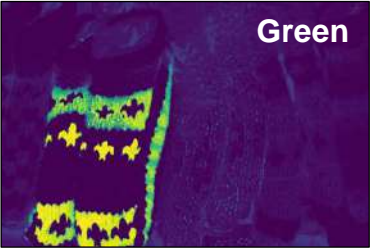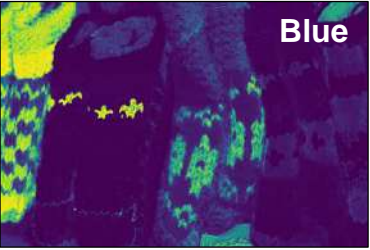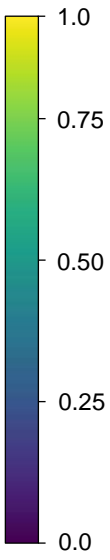

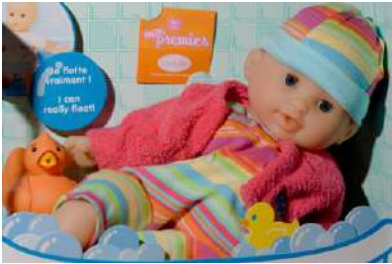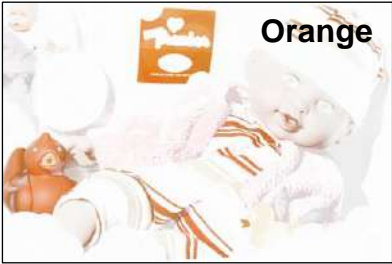

Orange

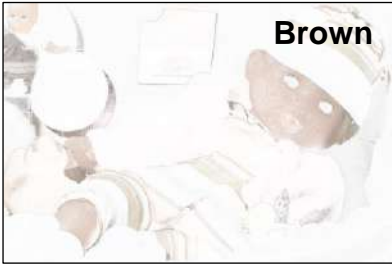

Brown

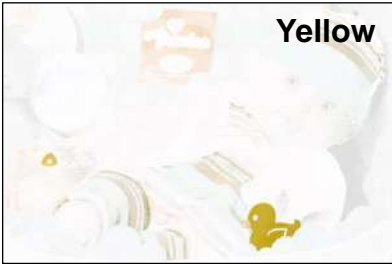

Yellow

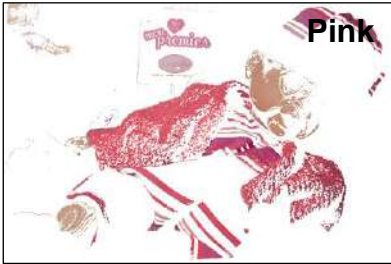

Pink

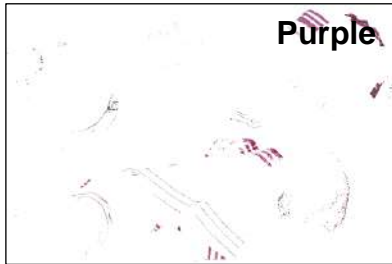

Purple

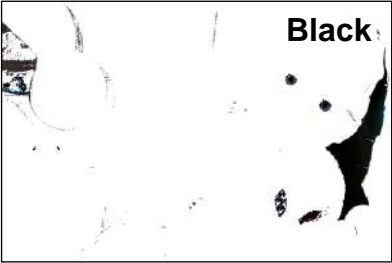

Black

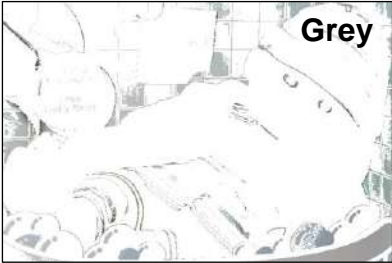

Grey

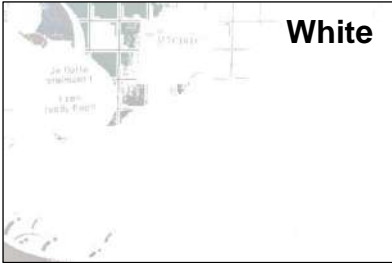

White

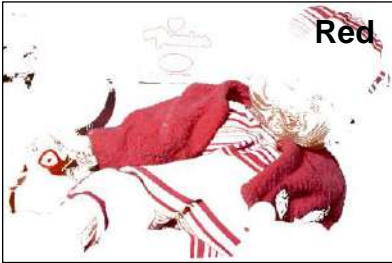

Red

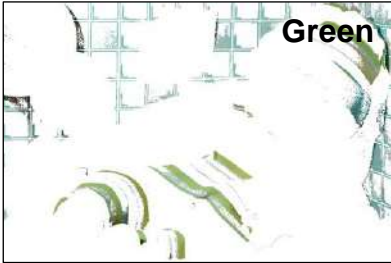

Green

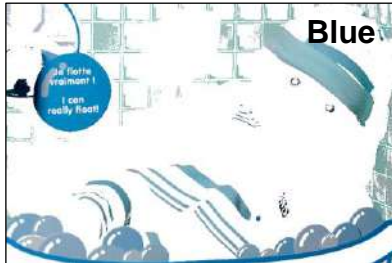

Blue



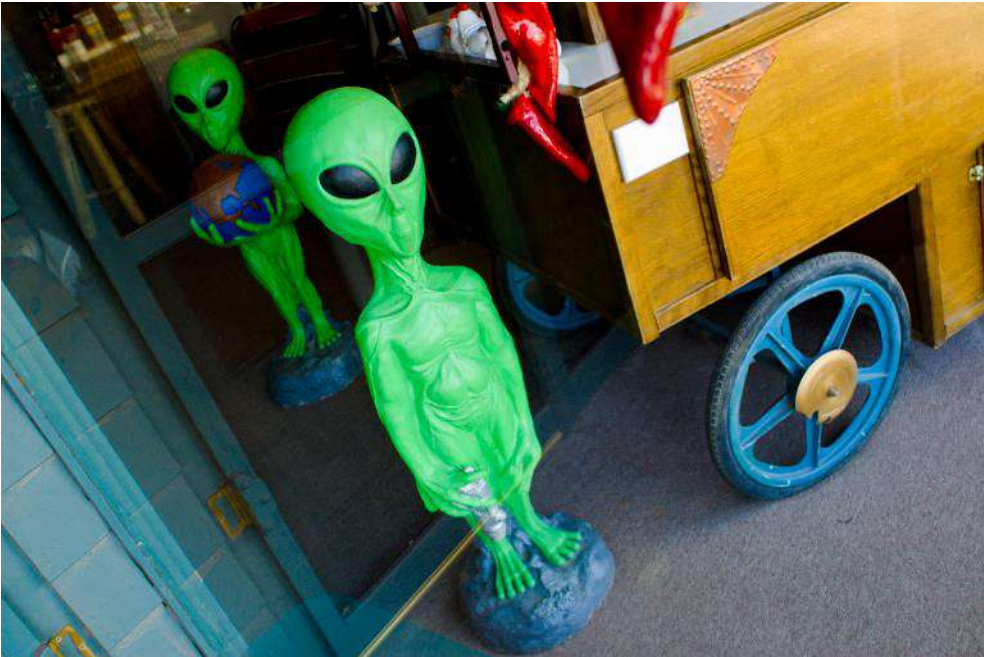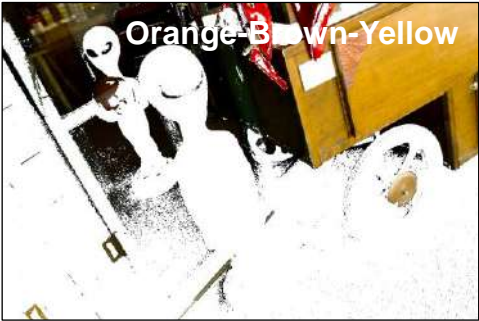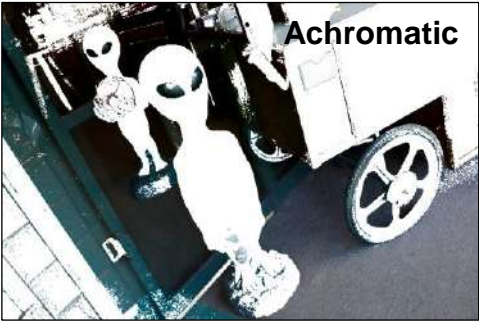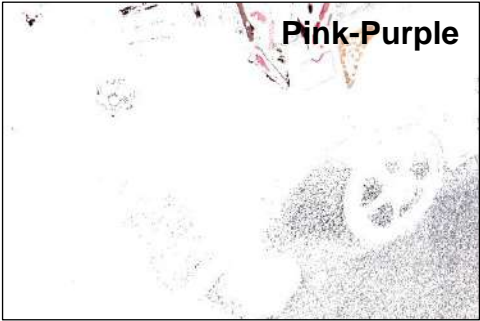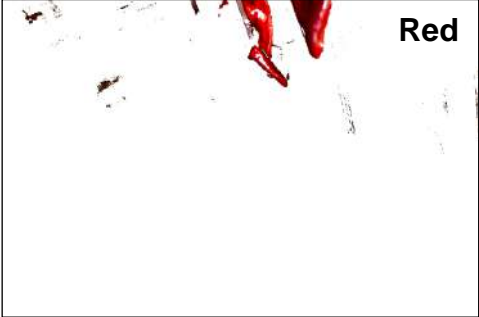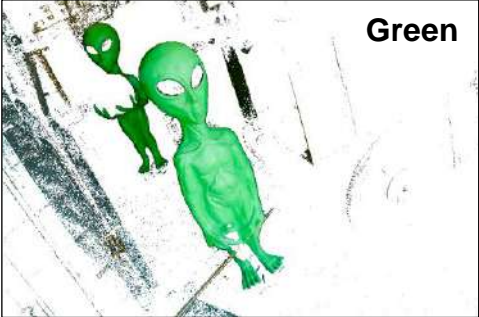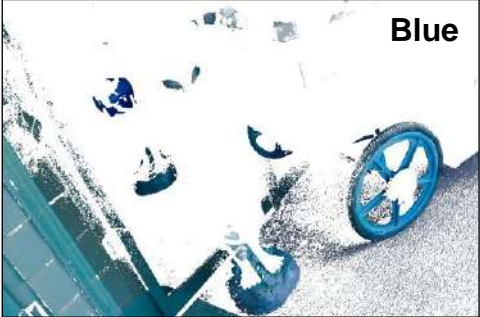

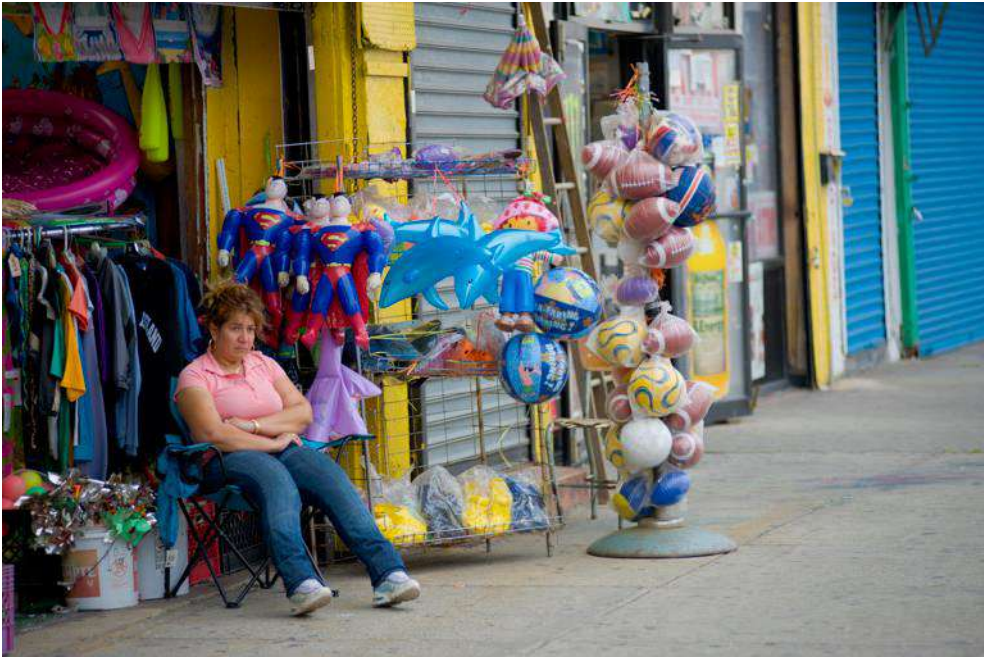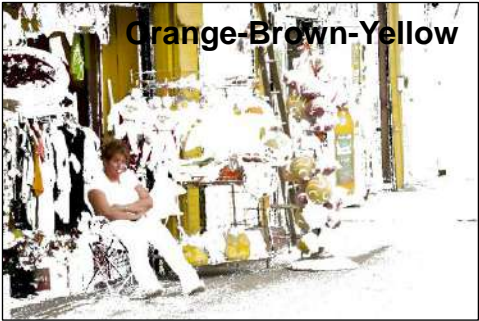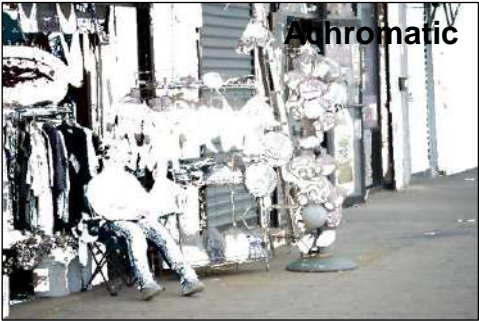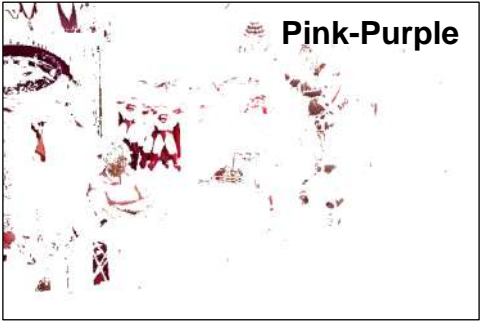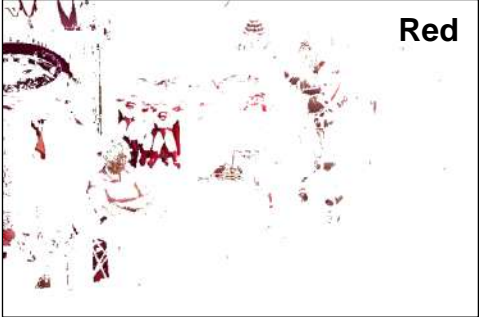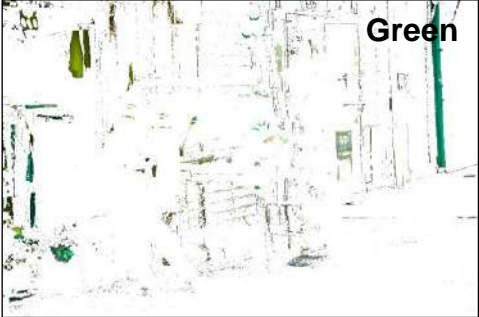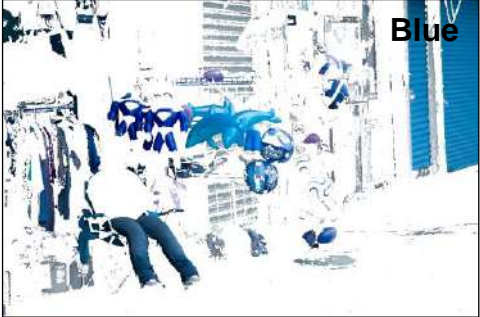

Supplement: Supplementary file 1 [file supplementary-color-naming.pdf]
